# Supplementary material for: Eye-Shield: Real-Time Protection of Mobile Device Screen Information from Shoulder Surfing
Source: arXiv:2308.03868 source file (2023-08-07)
Supplement: Supplementary file 1 [file fig_prototype_appendix.tex]

\begin{figure}[h]
\centering
  \centering
  \includegraphics[width=0.8\columnwidth]{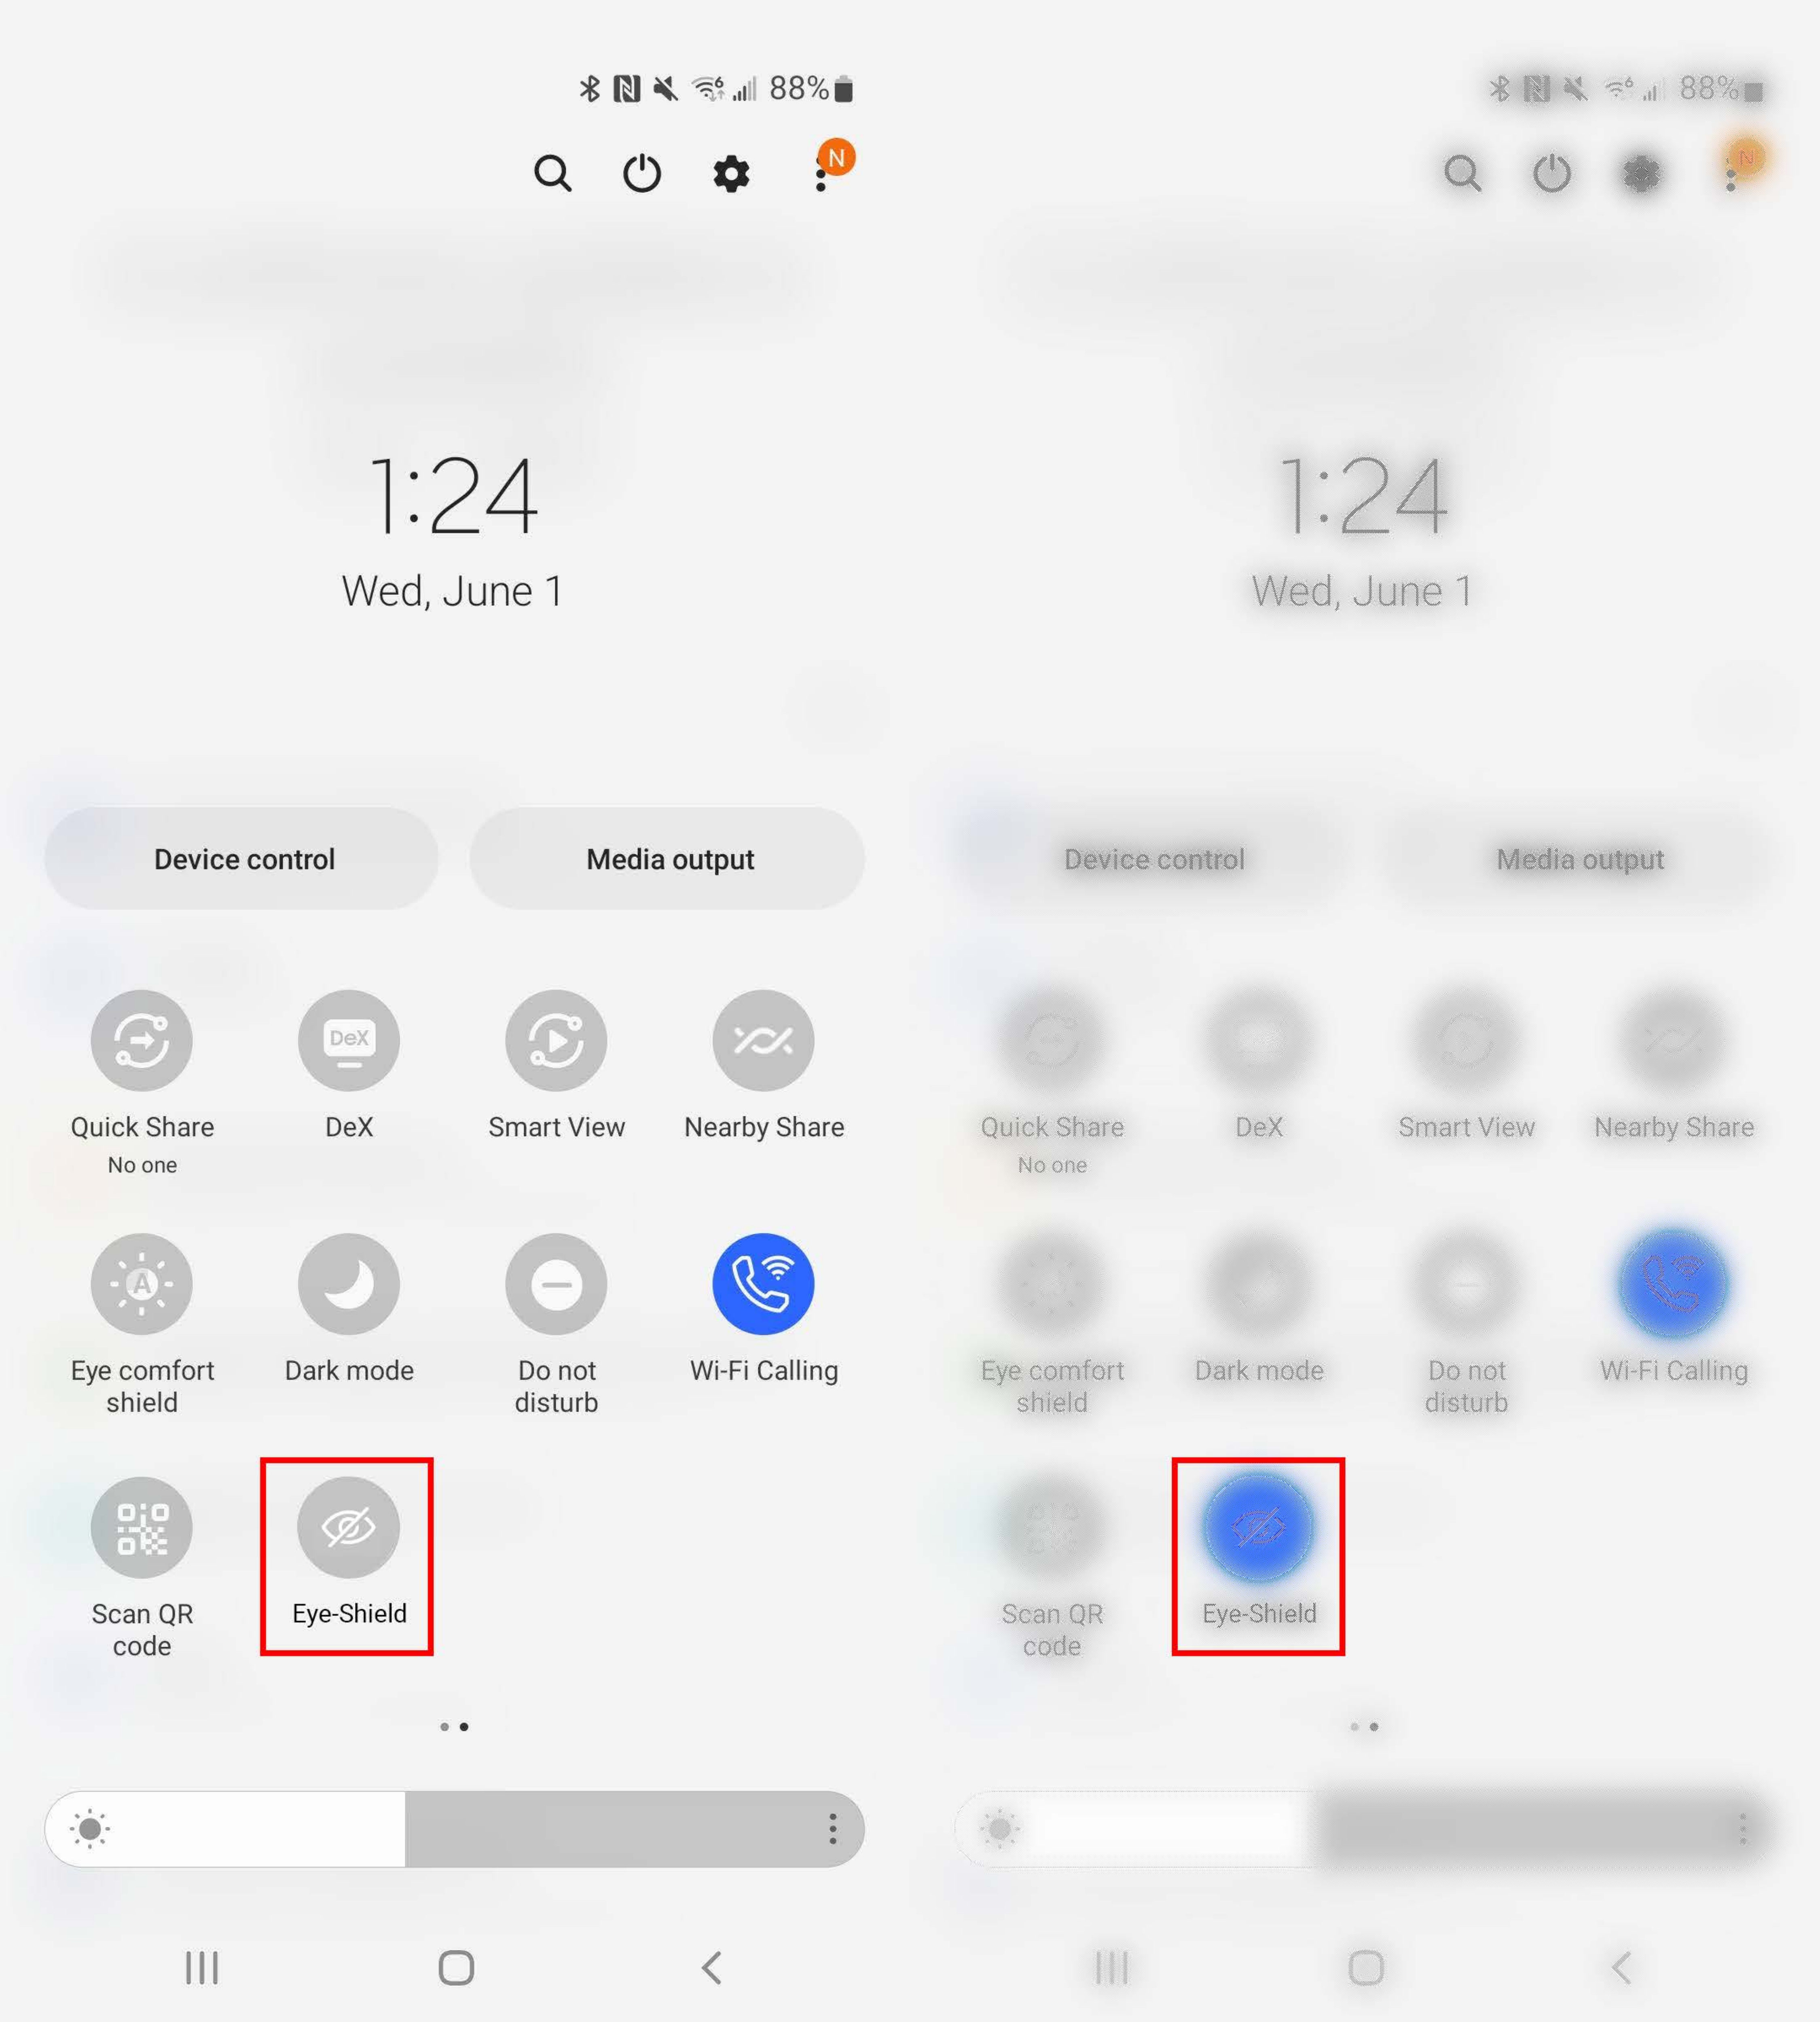}
%   \caption{Android}
  \caption{Android UI Prototype for toggling \name. The red box highlights the control for protecting the screen.}
  \label{fig:prototype_android}
\end{figure}
